# Supplementary material for: ICF-SRSR: Invertible scale-Conditional Function for Self-Supervised Real-world Single Image Super-Resolution
Source: arXiv:2307.12751 source file (2023-08-31)
Supplement: Supplementary file 1 [file loss.tex]

\begin{figure*}[t]
	\captionsetup[]{labelformat=empty}
	%\begin{center}

		% 			\begin{adjustbox}{width=\linewidth, center=\linewidth}
		\setlength\tabcolsep{0.05cm}
    \subfloat[Quantitative results.]{
    \footnotesize
    \begin{tabularx}{0.32 \linewidth}{>{\centering\arraybackslash}X
    >{\centering\arraybackslash}X >{\centering\arraybackslash}X c }
        \toprule
        \textbf{$\mathcal{L}^{\text{Cons}}$} & \textbf{$\mathcal{L}^{\text{Avg}}$} & \textbf{$\mathcal{L}^{\text{Pool}}$} &
        \textbf{PSNR}   \\ 
        %\textbf{A} & \textbf{B} & & \\
        %\cline{3-8}
        %&&time & iteration & time & iteration & time & %iteration  \\
        \midrule
        \textcolor{red}{\ding{55}} & \textcolor{ForestGreen}{\ding{51}} & \textcolor{red}{\ding{55}} & 28.97\\
        \textcolor{red}{\ding{55}} & \textcolor{red}{\ding{55}} &  \textcolor{ForestGreen}{\ding{51}} & 30.65\\
        \textcolor{ForestGreen}{\ding{51}} & \textcolor{red}{\ding{55}} & \textcolor{red}{\ding{55}} & 13.51 \\
        \textcolor{red}{\ding{55}} & \textcolor{ForestGreen}{\ding{51}} & \textcolor{ForestGreen}{\ding{51}} & 30.68\\       
         %\textcolor{ForestGreen}{\ding{51}} & \textcolor{ForestGreen}{\ding{51}} & \textcolor{red}{\ding{55}} & 26.55 \\
        \textcolor{ForestGreen}{\ding{51}} & \textcolor{ForestGreen}{\ding{51}} &  \textcolor{ForestGreen}{\ding{51}} & \textbf{37.01}\\
        \bottomrule
        \vspace{1mm}
    \end{tabularx}
    \label{tab:supp_loss}
    }
    \subfloat[Qualitative results. \label{tab:QualiKITTI}]{
        \footnotesize
		\begin{tabular}[b]{c c c}
				\includegraphics[width = .10\textwidth]
				{figures/supplement/S6/bird/ave.png.jpg}
				\includegraphics[width = .10\textwidth]
				{figures/supplement/S6/bird/pool.png.jpg}
				\includegraphics[width =.10\textwidth]
				{figures/supplement/S6/bird/cons.png.jpg}
				\includegraphics[width = .10\textwidth]
				{figures/supplement/S6/bird/-cons.png.jpg}
				\includegraphics[width = .10\textwidth]
				{figures/supplement/S6/bird/total.png.jpg}
				\includegraphics[width = .10\textwidth]
				{figures/supplement/S6/bird/gt.png.jpg}
				\vspace{1mm}
				\\
				\includegraphics[width = .10\textwidth]
				{figures/supplement/S6/butterfly/ave.png.jpg}
				\includegraphics[width = .10\textwidth]
				{figures/supplement/S6/butterfly/pool.png.jpg}
				\includegraphics[width =.10\textwidth]
				{figures/supplement/S6/butterfly/cons.png.jpg}
				\includegraphics[width = .10\textwidth]
				{figures/supplement/S6/butterfly/-cons.png.jpg}
				\includegraphics[width = .10\textwidth]
				{figures/supplement/S6/butterfly/total.png.jpg}
				\includegraphics[width = .10\textwidth]
				{figures/supplement/S6/butterfly/gt.png.jpg}
				\vspace{1mm}
				\\  
			\setcounter{subfigure}{0}
			\begin{minipage}{.10\textwidth}
            \centering
            \includegraphics[width=1\linewidth]{figures/supplement/S6/woman/ave.png.jpg}
            \vspace{\abovecaptionskip}%
            \tiny $\mathcal{L}^{\text{Avg}}$
            \end{minipage}
            
            \begin{minipage}{.10\textwidth}
            \centering
            \includegraphics[width=1\linewidth]{figures/supplement/S6/woman/pool.png.jpg}
            \vspace{\abovecaptionskip}%
            \tiny $\mathcal{L}^{\text{Pool}}$
            \end{minipage}
            
            \begin{minipage}{.10\textwidth}
            \centering
            \includegraphics[width=1\linewidth]{figures/supplement/S6/woman/cons.png.jpg}
            \vspace{\abovecaptionskip}%
            \tiny $\mathcal{L}^{\text{Cons}}$
            \end{minipage}
            
            \begin{minipage}{.10\textwidth}
            \centering
            \includegraphics[width=1\linewidth]{figures/supplement/S6/woman/-cons.png.jpg}
            \vspace{\abovecaptionskip}%
            \tiny $\mathcal{L}^{\text{Avg}}+\mathcal{L}^{\text{Pool}}
            \end{minipage}
            
            \begin{minipage}{.10\textwidth}
            \centering
            \includegraphics[width=1\linewidth]{figures/supplement/S6/woman/total.png.jpg}
            \vspace{\abovecaptionskip}%
            \tiny $\mathcal{L}^{\text{Total}}$
            \end{minipage}

            \begin{minipage}{.10\textwidth}
            \centering
            \includegraphics[width=1\linewidth]{figures/supplement/S6/woman/gt.png.jpg}
            \vspace{\abovecaptionskip}%
            \tiny GT~(HR)
            \end{minipage}
            \setcounter{subfigure}{1}
	    \end{tabular}}
	%\setlength{\abovecaptionskip}{0cm}
	%\vspace{1mm}
	%\captionsetup{justification=raggedright,singlelinecheck=false}
	\caption{\textbf{Evaluation of the effect of loss functions.} We show the importance of  $\mathcal{L}^{\text{Avg}}$ and  $\mathcal{L}^{\text{Pool}}$ to ease the convergence by constraining the search space and  $\mathcal{L}^{\text{Cons}}$ to achieve satisfactory SR images (a) quantitatively and (b) qualitatively.
	}
	\label{fig:supp_loss}
	\vspace{2mm}
\end{figure*}
