# Supplementary material for: ICF-SRSR: Invertible scale-Conditional Function for Self-Supervised Real-world Single Image Super-Resolution
Source: arXiv:2307.12751 source file (2023-08-31)

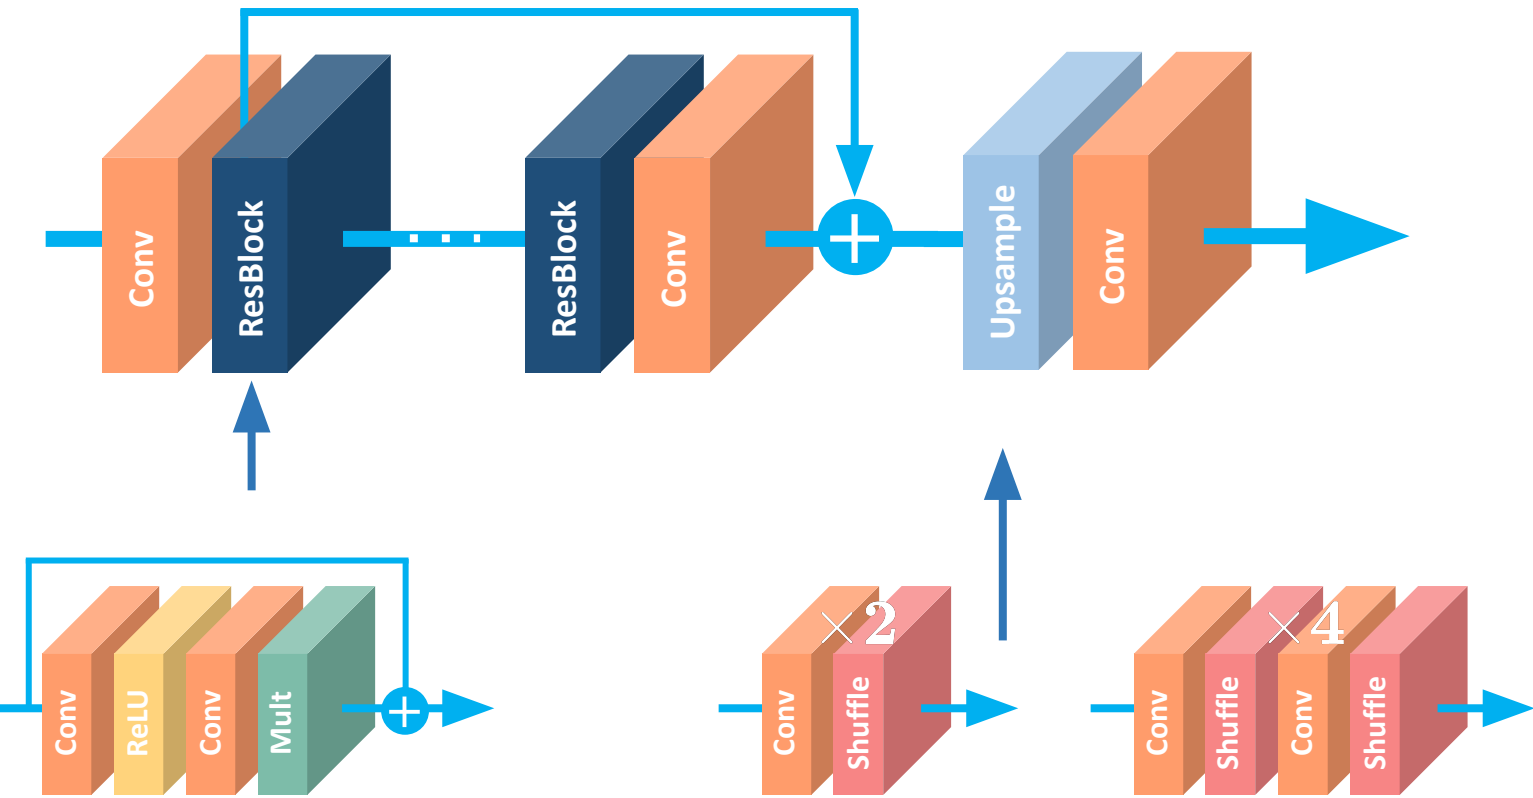

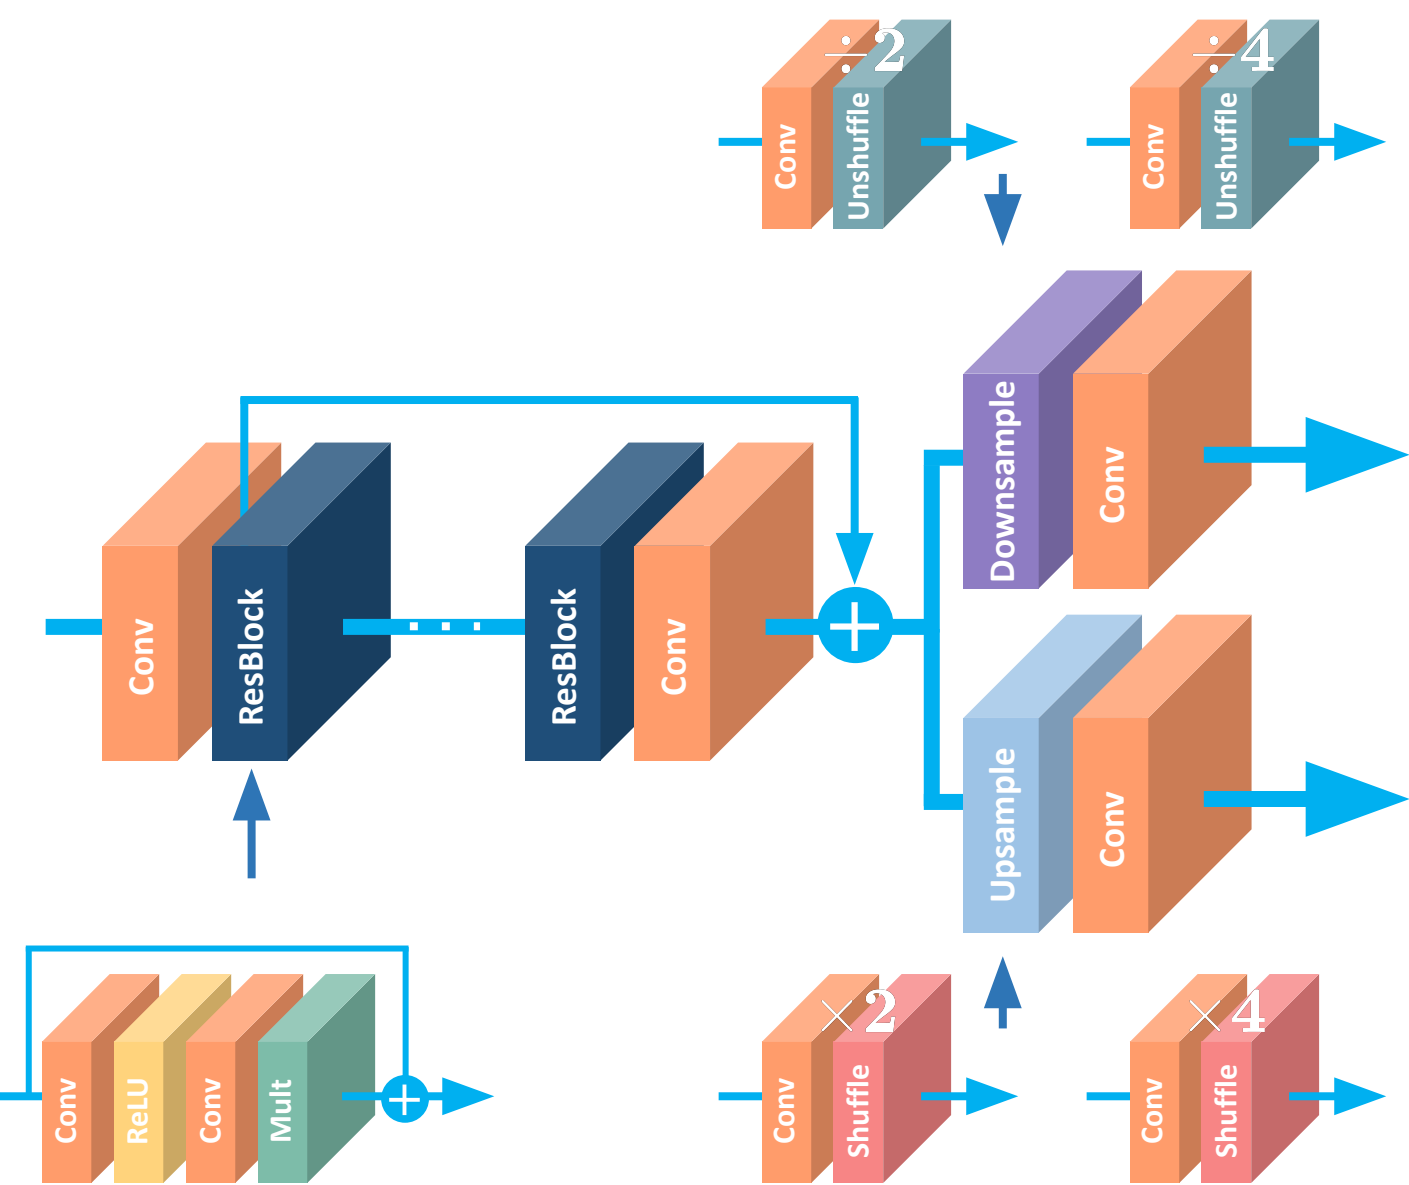

Supplement: Supplementary file 2 [file EDSR.pdf]
