# Supplementary material for: ICF-SRSR: Invertible scale-Conditional Function for Self-Supervised Real-world Single Image Super-Resolution
Source: arXiv:2307.12751 source file (2023-08-31)
Supplement: Supplementary file 3 [file down.tex]

\begin{figure*}
     \centering
     %%%%%%%%%%%%%%%%%%%%%%%%%%% Set14 %%%%%%%%%%%%%%%%%%%%%%%%%%
     \begin{subfigure}[b]{0.19\textwidth}
         \centering
         \includegraphics[width=\textwidth]{figures/supplement/S7/set14/input.png}
     \end{subfigure}
     \hfill
     \begin{subfigure}[b]{0.19\textwidth}
         \centering
         \includegraphics[width=\textwidth]{figures/supplement/S7/set14/gn.png}
     \end{subfigure}
     \hfill
     \begin{subfigure}[b]{0.19\textwidth}
         \centering
         \includegraphics[width=\textwidth]{figures/supplement/S7/set14/gb.png}
     \end{subfigure}
     \hfill
     \begin{subfigure}[b]{0.19\textwidth}
         \centering
         \includegraphics[width=\textwidth]{figures/supplement/S7/set14/b.png}
     \end{subfigure}
     \hfill
     \begin{subfigure}[b]{0.19\textwidth}
         \centering
         \includegraphics[width=\textwidth]{figures/supplement/S7/set14/Ours.png}
     \end{subfigure}
     \\
    %%%%%%%%%%%%%%%%%%%%%%%%%%% B100 %%%%%%%%%%%%%%%%%%%%%%%%%%
     \begin{subfigure}[b]{0.19\textwidth}
         \centering
         \includegraphics[width=\textwidth]{figures/supplement/S7/b100/input.png}
     \end{subfigure}
     \hfill    
     \begin{subfigure}[b]{0.19\textwidth}
         \centering
         \includegraphics[width=\textwidth]{figures/supplement/S7/b100/gn.png}
     \end{subfigure}
     \hfill
     \begin{subfigure}[b]{0.19\textwidth}
         \centering
         \includegraphics[width=\textwidth]{figures/supplement/S7/b100/gb.png}
     \end{subfigure}
     \hfill
     \begin{subfigure}[b]{0.19\textwidth}
         \centering
         \includegraphics[width=\textwidth]{figures/supplement/S7/b100/b.png}
     \end{subfigure}
     \hfill
     \begin{subfigure}[b]{0.19\textwidth}
         \centering
         \includegraphics[width=\textwidth]{figures/supplement/S7/b100/Ours.png}
     \end{subfigure}
     \\
     %%%%%%%%%%%%%%%%%%%%%%%%%%% Urban100 %%%%%%%%%%%%%%%%%%%%%%%%%%
     \begin{subfigure}[b]{0.19\textwidth}
         \centering
         \includegraphics[width=\textwidth]{figures/supplement/S7/urban100/input.png}
     \end{subfigure}
     \hfill
     \begin{subfigure}[b]{0.19\textwidth}
         \centering
         \includegraphics[width=\textwidth]{figures/supplement/S7/urban100/gn.png}
     \end{subfigure}
     \hfill
     \begin{subfigure}[b]{0.19\textwidth}
         \centering
         \includegraphics[width=\textwidth]{figures/supplement/S7/urban100/gb.png}
     \end{subfigure}
     \hfill
     \begin{subfigure}[b]{0.19\textwidth}
         \centering
         \includegraphics[width=\textwidth]{figures/supplement/S7/urban100/b.png}
     \end{subfigure}
     \hfill
     \begin{subfigure}[b]{0.19\textwidth}
         \centering
         \includegraphics[width=\textwidth]{figures/supplement/S7/urban100/Ours.png}
     \end{subfigure}
     \\
     %%%%%%%%%%%%%%%%%%%%%%%%%%% RealSR %%%%%%%%%%%%%%%%%%%%%%%%%%
     \begin{subfigure}[b]{0.19\textwidth}
         \centering
         \includegraphics[width=\textwidth]{figures/supplement/S7/realsr/input.png}
         \caption*{\tiny LR~(Input)}
     \end{subfigure}
     \hfill
     \begin{subfigure}[b]{0.19\textwidth}
         \centering
         \includegraphics[width=\textwidth]{figures/supplement/S7/realsr/gn.png}
         \caption*{\tiny LLR~(Gaussian+nearest)}
     \end{subfigure}
     \hfill
     \begin{subfigure}[b]{0.19\textwidth}
         \centering
         \includegraphics[width=\textwidth]{figures/supplement/S7/realsr/gb.png}
         \caption*{\tiny LLR~(Gaussian+bicubic)}
     \end{subfigure}
     \hfill
     \begin{subfigure}[b]{0.19\textwidth}
         \centering
         \includegraphics[width=\textwidth]{figures/supplement/S7/realsr/b.png}
         \caption*{\tiny LLR~(bicubic)}
     \end{subfigure}
     \hfill
     \begin{subfigure}[b]{0.19\textwidth}
         \centering
         \includegraphics[width=\textwidth]{figures/supplement/S7/realsr/ours.png}
         \caption*{\tiny LLR~(Ours)}
     \end{subfigure}
     \\
        \caption{
        \textbf{Qualitative comparisons of various down-sampling operators.} 
        }
        \label{fig:supp_down}
\end{figure*}
