# Supplementary material for: ICF-SRSR: Invertible scale-Conditional Function for Self-Supervised Real-world Single Image Super-Resolution
Source: arXiv:2307.12751 source file (2023-08-31)
Supplement: Supplementary file 4 [file realsr_x2.tex]

\begin{figure*}[t]
	\captionsetup[subfloat]{labelformat=empty}
	%\begin{center}
		\newcommand{\rowArg}{.68cm}
		\newcommand{\fullSize}{2.4cm}
		\newcommand{\patchSize}{1.24cm}
		% 			\begin{adjustbox}{width=\linewidth, center=\linewidth}
		\setlength\tabcolsep{0.0cm}
		\begin{tabular}[b]{c c c}
			\multicolumn{2}{c}{\multirow{2}{*}[\rowArg]{
					\subfloat[Input~(LR)]
					% 			{\includegraphics[width = \fullSize, height = \fullSize]
					{\includegraphics[height=\fullSize]
						{example-image-a}}}} &
			\subfloat[\centering \tiny Bicubic ]{
				\includegraphics[width = \patchSize]
				{example-image-a}} 
			\subfloat[\centering \tiny    ]{
				\includegraphics[width = \patchSize]
				{example-image-a}} 
			\subfloat[\centering \tiny    ]{
				\includegraphics[width = \patchSize]
				{example-image-a}} \\  & &

			\subfloat[\centering  \tiny  ]{
				\includegraphics[width = \patchSize]
				{example-image-a}}
			\subfloat[\centering  \tiny \textbf{IMF-SRSR}~(Ours) ]{
				\includegraphics[width = \patchSize]
				{example-image-a}}
				%\vspace{2.25mm}
			\subfloat[\centering \tiny GT~(HR)]{
				\includegraphics[width = \patchSize]
				{example-image-a}}
	\end{tabular}
	%%%%%%%%%%%%%%%%%%%%%%%%%%%%%%%%%
		\begin{tabular}[b]{c c c}
			\multicolumn{2}{c}{\multirow{2}{*}[\rowArg]{
					\subfloat[Input~(LR)]
					% 			{\includegraphics[width = \fullSize, height = \fullSize]
					{\includegraphics[height=\fullSize]
						{example-image-a}}}} &
			\subfloat[\centering \tiny Bicubic ]{
				\includegraphics[width = \patchSize]
				{example-image-a}} 
			\subfloat[\centering \tiny    ]{
				\includegraphics[width = \patchSize]
				{example-image-a}} 
			\subfloat[\centering \tiny    ]{
				\includegraphics[width = \patchSize]
				{example-image-a}} \\  & &

			\subfloat[\centering  \tiny  ]{
				\includegraphics[width = \patchSize]
				{example-image-a}}
			\subfloat[\centering  \tiny \textbf{IMF-SRSR}~(Ours) ]{
				\includegraphics[width = \patchSize]
				{example-image-a}}
				%\vspace{2.25mm}
			\subfloat[\centering \tiny GT~(HR)]{
				\includegraphics[width = \patchSize]
				{example-image-a}}
	\end{tabular}
	\\
		\begin{tabular}[b]{c c c}
			\multicolumn{2}{c}{\multirow{2}{*}[\rowArg]{
					\subfloat[Input~(LR)]
					% 			{\includegraphics[width = \fullSize, height = \fullSize]
					{\includegraphics[height=\fullSize]
						{example-image-a}}}} &
			\subfloat[\centering \tiny Bicubic ]{
				\includegraphics[width = \patchSize]
				{example-image-a}} 
			\subfloat[\centering \tiny    ]{
				\includegraphics[width = \patchSize]
				{example-image-a}} 
			\subfloat[\centering \tiny    ]{
				\includegraphics[width = \patchSize]
				{example-image-a}} \\  & &

			\subfloat[\centering  \tiny  ]{
				\includegraphics[width = \patchSize]
				{example-image-a}}
			\subfloat[\centering  \tiny \textbf{IMF-SRSR}~(Ours) ]{
				\includegraphics[width = \patchSize]
				{example-image-a}}
				%\vspace{2.25mm}
			\subfloat[\centering \tiny GT~(HR)]{
				\includegraphics[width = \patchSize]
				{example-image-a}}
	\end{tabular}
	%%%%%%%%%%%%%%%%%%%%%%%%%%%%%%%%%
		\begin{tabular}[b]{c c c}
			\multicolumn{2}{c}{\multirow{2}{*}[\rowArg]{
					\subfloat[Input~(LR)]
					% 			{\includegraphics[width = \fullSize, height = \fullSize]
					{\includegraphics[height=\fullSize]
						{example-image-a}}}} &
			\subfloat[\centering \tiny Bicubic ]{
				\includegraphics[width = \patchSize]
				{example-image-a}} 
			\subfloat[\centering \tiny    ]{
				\includegraphics[width = \patchSize]
				{example-image-a}} 
			\subfloat[\centering \tiny    ]{
				\includegraphics[width = \patchSize]
				{example-image-a}} \\  & &

			\subfloat[\centering  \tiny  ]{
				\includegraphics[width = \patchSize]
				{example-image-a}}
			\subfloat[\centering  \tiny \textbf{IMF-SRSR}~(Ours) ]{
				\includegraphics[width = \patchSize]
				{example-image-a}}
				%\vspace{2.25mm}
			\subfloat[\centering \tiny GT~(HR)]{
				\includegraphics[width = \patchSize]
				{example-image-a}}
	\end{tabular}
	\setlength{\abovecaptionskip}{0cm}
	%\vspace{-2mm}
	%\captionsetup{justification=raggedright,singlelinecheck=false}
	
	\caption{\textbf{Qualitative results on the RealSR-V3~\cite{} dataset for scale $\times2$.} 
	}
	\label{fig:supp_realsx2}
	%\vspace{2mm}
\end{figure*}
